# Supplementary material for: Data Feedback Loops: Model-driven Amplification of Dataset Biases
Source: arXiv:2209.03942 source file (2022-09-08)
Supplement: Supplementary file 1 [file cifar-intervention.tex]

\begin{figure*}[t!]
    \centering
    \includegraphics[width=0.8\textwidth]{figures/cifar_intervention.pdf}
    \caption{
        Results of data feedback (Algorithm \ref{alg:main}) on the CIFAR-10 dataset [CITE]
        with 20\% uniform label noise.
        The initial dataset size is 20k, and each round adds 5k additional samples,
        4.5k of which are model-labeled samples.
        The dataset is randomly subsampled to 20k examples at each round.
        We train a BaiduNet9 from scratch at each round.
        We explore two experimental settings:
        (\textbf{blue}) the standard setting where model predictions
        are the class with largest score, and 
        (\textbf{orange}) an intervention where after training each round,
        the model is temperature-calibrated [CITE] on a separate held-out test set,
        and predictions are then sampled from the softmax score distribution.
        We display the empirical accuracies of the two models, shown with the mean
        and standard deviation over 3 random seeds.
        The calibrated and softmax-sampled model quickly loses 
        accuracy.
    } 
    \label{fig:cifar-intervention}
\end{figure*}

We also present another intervention inspired by our stability analysis,
this time to take a stable system and make it unstable.
Experiments in Section \ref{sec:vision} showed that
interpolating image classifiers on CIFAR are generally stable.
To make the model unstable, we modify the prediction procedure:
instead of assigning the prediction to the class 
with the largest score,
we first temperature-calibrate [CITE] the model 
on a separate held-out test set,
and then sample from the softmax distribution
at prediction time.
Sampling ensures that the model is no longer interpolating,
and calibration is needed to ensure that the softmax distributions
are not peaky (otherwise sampling would behave similarly to argmax).
\thc{
  This is going to get confusing-  reader will go. wait i thought sampling=good?
  We need a simpler way to explain why we're sampling (we want a \emph{terrible} sampler)
}
We run this procedure on a dataset with 20\% uniform label noise
and plot the results in Figure \ref{fig:cifar-intervention}.

On Figure \ref{fig:cifar-intervention}, we compare the standard model prediction setting
to the calibrate-then-sample model prediction setting
and plot accuracies for both over time under data feedback.
We observe that the calibrate-then sample model quickly degrades in accuracy,
reaching 73\% accuracy after 85 feedback rounds,
versus the standard model which reaches 82\% accuracy,
which is near the dataset-level accuracy.
\rtc{Kind of unhappy with the figure results - looks like blue also amplifies,
  just in the reverse direction. even though it stabilizes to near the dataset level accuracy}
Though running this procedure provides no utility,
it demonstrates another way that modifying a model 
to not behave like a sampler can result in bias amplification.
\rtc{Does the model really not behave like a sampler though? Seems like
it does behave like a sampler, just that it's a worse sampler than the 
standard model. So all this intervention does is reduce the quality
of the model, but it's still a sampler. Thoughts (?)}
\thc{yes, see comment above}
